# Supplementary material for: Statistical Signatures of Nanoflare Activity. III. Evidence of Enhanced Nanoflaring Rates in Fully Convective stars as Observed by the NGTS
Source: arXiv:2309.10035 source file (2023-09-18)
Supplement: Supplementary file 1 [file Appendix.tex]

\appendix

\section{Appendix information}

Appendices can be broken into separate sections just like in the main text.
The only difference is that each appendix section is indexed by a letter
(A, B, C, etc.) instead of a number.  Likewise numbered equations have
the section letter appended.  Here is an equation as an example.

\begin{equation}
I = \frac{1}{1 + d_{1}^{P (1 + d_{2} )}}
\end{equation}

Appendix tables and figures should not be numbered like equations. Instead
they should continue the sequence from the main article body.

\section{Author publication charges} \label{sec:pubcharge}

Finally some information about the AAS Journal's publication charges.
In April 2011 the traditional way of calculating author charges based on 
the number of printed pages was changed.  The reason for the change
was due to a recognition of the growing number of article items that could not 
be represented in print. Now author charges are determined by a number of
digital ``quanta''.  A single quantum is 350 words, one figure, one table,
and one enhanced digital item.  For the latter this includes machine readable
tables, figure sets, animations, and interactive figures.  The current cost
for the different quanta types is available at 
\url{https://journals.aas.org/article-charges-and-copyright/#author_publication_charges}. 
Authors may use the ApJL length calculator to get a {\tt rough} estimate of 
the number of word and float quanta in their manuscript. The calculator 
is located at \url{https://authortools.aas.org/ApJL/betacountwords.html}.

\section{Rotating tables} \label{sec:rotate}

The process of rotating tables into landscape mode is slightly different in
\aastex v6.3. Instead of the {\tt\string\rotate} command, a new environment
has been created to handle this task. To place a single page table in a
landscape mode start the table portion with
{\tt\string\begin\{rotatetable\}} and end with
{\tt\string\end\{rotatetable\}}.

Tables that exceed a print page take a slightly different environment since
both rotation and long table printing are required. In these cases start
with {\tt\string\begin\{longrotatetable\}} and end with
{\tt\string\end\{longrotatetable\}}. Table \ref{chartable} is an
example of a multi-page, rotated table. The {\tt\string\movetabledown}
command can be used to help center extremely wide, landscape tables. The
command {\tt\string\movetabledown=1in} will move any rotated table down 1
inch. 

\begin{longrotatetable}
\begin{deluxetable*}{lllrrrrrrll}
\tablecaption{Observable Characteristics of 
Galactic/Magellanic Cloud novae with X-ray observations\label{chartable}}
\tablewidth{700pt}
\tabletypesize{\scriptsize}
\tablehead{
\colhead{Name} & \colhead{V$_{max}$} & 
\colhead{Date} & \colhead{t$_2$} & 
\colhead{FWHM} & \colhead{E(B-V)} & 
\colhead{N$_H$} & \colhead{Period} & 
\colhead{D} & \colhead{Dust?} & \colhead{RN?} \\ 
\colhead{} & \colhead{(mag)} & \colhead{(JD)} & \colhead{(d)} & 
\colhead{(km s$^{-1}$)} & \colhead{(mag)} & \colhead{(cm$^{-2}$)} &
\colhead{(d)} & \colhead{(kpc)} & \colhead{} & \colhead{}
} 
\startdata
CI Aql & 8.83 (1) & 2451665.5 (1) & 32 (2) & 2300 (3) & 0.8$\pm0.2$ (4) & 1.2e+22 & 0.62 (4) & 6.25$\pm5$ (4) & N & Y \\
{\bf CSS081007} & \nodata & 2454596.5 & \nodata & \nodata & 0.146 & 1.1e+21 & 1.77 (5) & 4.45$\pm1.95$ (6) & \nodata & \nodata \\
GQ Mus & 7.2 (7) & 2445352.5 (7) & 18 (7) & 1000 (8) & 0.45 (9) & 3.8e+21  & 0.059375 (10) & 4.8$\pm1$ (9) & N (7) & \nodata \\
IM Nor & 7.84 (11) & 2452289 (2) & 50 (2) & 1150 (12) & 0.8$\pm0.2$ (4) & 8e+21 & 0.102 (13) & 4.25$\pm3.4$ (4) & N & Y \\
{\bf KT Eri} & 5.42 (14) & 2455150.17 (14) & 6.6 (14) & 3000 (15) & 0.08 (15) & 5.5e+20 & \nodata & 6.5 (15) & N & M \\
{\bf LMC 1995} & 10.7 (16) & 2449778.5 (16) & 15$\pm2$ (17) & \nodata & 0.15 (203) & 7.8e+20  & \nodata & 50 & \nodata & \nodata \\
LMC 2000 & 11.45 (18) & 2451737.5 (18) & 9$\pm2$ (19) & 1700 (20) & 0.15 (203) & 7.8e+20  & \nodata & 50 & \nodata & \nodata \\
{\bf LMC 2005} & 11.5 (21) & 2453700.5 (21) & 63 (22) & 900 (23) & 0.15 (203) & 1e+21 & \nodata & 50  & M (24) & \nodata \\
{\bf LMC 2009a} & 10.6 (25) & 2454867.5 (25) & 4$\pm1$  & 3900 (25) & 0.15 (203)  & 5.7e+20 & 1.19 (26) & 50 & N & Y \\
{\bf SMC 2005} & 10.4 (27) & 2453588.5 (27) & \nodata & 3200 (28) & \nodata & 5e+20  & \nodata & 61 & \nodata & \nodata \\
{\bf QY Mus} & 8.1 (29) & 2454739.90 (29) & 60:  & \nodata & 0.71 (30) & 4.2e+21  & \nodata & \nodata & M & \nodata \\
{\bf RS Oph} & 4.5 (31) & 2453779.44 (14) & 7.9 (14) & 3930 (31) & 0.73 (32) & 2.25e+21 & 456 (33) & 1.6$\pm0.3$ (33) & N (34) & Y \\
{\bf U Sco} & 8.05 (35) & 2455224.94 (35) & 1.2 (36) & 7600 (37) & 0.2$\pm0.1$ (4) & 1.2e+21 & 1.23056 (36) & 12$\pm2$ (4) & N & Y \\
{\bf V1047 Cen} & 8.5 (38) & 2453614.5 (39) & 6 (40) & 840 (38) & \nodata & 1.4e+22  & \nodata & \nodata & \nodata & \nodata \\
{\bf V1065 Cen} & 8.2 (41) & 2454123.5 (41) & 11 (42) & 2700 (43) & 0.5$\pm0.1$ (42) & 3.75e+21 & \nodata & 9.05$\pm2.8$ (42) & Y (42) & \nodata \\
V1187 Sco & 7.4 (44) & 2453220.5 (44) & 7: (45) & 3000 (44) & 1.56 (44) & 8.0e+21 & \nodata & 4.9$\pm0.5$ (44) & N & \nodata \\
{\bf V1188 Sco} & 8.7 (46) & 2453577.5 (46) & 7 (40) & 1730 (47) & \nodata & 5.0e+21  & \nodata & 7.5 (39) & \nodata & \nodata \\
{\bf V1213 Cen} & 8.53 (48) & 2454959.5 (48) & 11$\pm2$ (49) & 2300 (50) & 2.07 (30) & 1.0e+22 & \nodata & \nodata & \nodata & \nodata \\
{\bf V1280 Sco} & 3.79 (51) & 2454147.65 (14) & 21 (52) & 640 (53) & 0.36 (54) & 1.6e+21  & \nodata & 1.6$\pm0.4$ (54) & Y (54) & \nodata \\
{\bf V1281 Sco} & 8.8 (55) & 2454152.21 (55) & 15:& 1800 (56) & 0.7 (57) & 3.2e+21 & \nodata & \nodata & N & \nodata \\
{\bf V1309 Sco} & 7.1 (58) & 2454714.5 (58) & 23$\pm2$ (59) & 670 (60) & 1.2 (30) & 4.0e+21 & \nodata & \nodata & \nodata & \nodata \\
{\bf V1494 Aql} & 3.8 (61) & 2451515.5 (61) & 6.6$\pm0.5$ (61) & 1200 (62) & 0.6 (63) & 3.6e+21  & 0.13467 (64) & 1.6$\pm0.1$ (63) & N & \nodata \\
{\bf V1663 Aql} & 10.5 (65) & 2453531.5 (65) & 17 (66) & 1900 (67) & 2: (68) & 1.6e+22  & \nodata & 8.9$\pm3.6$ (69) & N & \nodata \\
V1974 Cyg & 4.3 (70) & 2448654.5 (70) & 17 (71) & 2000 (19) & 0.36$\pm0.04$ (71) & 2.7e+21  & 0.081263 (70) & 1.8$\pm0.1$ (72) & N & \nodata \\
{\bf V2361 Cyg} & 9.3 (73) & 2453412.5 (73) & 6 (40) & 3200 (74) & 1.2: (75) & 7.0e+21 & \nodata & \nodata & Y (40) & \nodata \\
{\bf V2362 Cyg} & 7.8 (76) & 2453831.5 (76) & 9 (77) & 1850 (78) & 0.575$\pm0.015$ (79) & 4.4e+21  & 0.06577 (80) & 7.75$\pm3$ (77) & Y (81) & \nodata \\
{\bf V2467 Cyg} & 6.7 (82) & 2454176.27 (82) & 7 (83) & 950 (82) & 1.5 (84) & 1.4e+22  & 0.159 (85) & 3.1$\pm0.5$ (86) & M (87) & \nodata \\
{\bf V2468 Cyg} & 7.4 (88) & 2454534.2 (88) & 10: & 1000 (88) & 0.77 (89) & 1.0e+22  & 0.242 (90) & \nodata & N & \nodata \\
{\bf V2491 Cyg} & 7.54 (91) & 2454567.86 (91) & 4.6 (92) & 4860 (93) & 0.43 (94) & 4.7e+21  & 0.09580: (95) & 10.5 (96) & N & M \\
V2487 Oph & 9.5 (97) & 2450979.5 (97) & 6.3 (98) & 10000 (98) & 0.38$\pm0.08$ (98) & 2.0e+21 & \nodata & 27.5$\pm3$ (99) & N (100) & Y (101) \\
{\bf V2540 Oph} & 8.5 (102) & 2452295.5 (102) & \nodata & \nodata & \nodata & 2.3e+21 & 0.284781 (103) & 5.2$\pm0.8$ (103) & N & \nodata \\
V2575 Oph & 11.1 (104) & 2453778.8 (104) & 20: & 560 (104) & 1.4 (105) & 3.3e+21 & \nodata & \nodata & N (105) & \nodata \\
{\bf V2576 Oph} & 9.2 (106) & 2453832.5 (106) & 8: & 1470 (106) & 0.25 (107) & 2.6e+21  & \nodata & \nodata & N & \nodata \\
{\bf V2615 Oph} & 8.52 (108) & 2454187.5 (108) & 26.5 (108) & 800 (109) & 0.9 (108) & 3.1e+21  & \nodata & 3.7$\pm0.2$ (108) & Y (110) & \nodata \\
{\bf V2670 Oph} & 9.9 (111) & 2454613.11 (111) & 15: & 600 (112) & 1.3: (113) & 2.9e+21  & \nodata & \nodata & N (114) & \nodata \\
{\bf V2671 Oph} & 11.1 (115) & 2454617.5 (115) & 8: & 1210 (116) & 2.0 (117) & 3.3e+21  & \nodata & \nodata & M (117) & \nodata \\
{\bf V2672 Oph} & 10.0 (118) & 2455060.02 (118) & 2.3 (119) & 8000 (118) & 1.6$\pm0.1$ (119) & 4.0e+21  & \nodata & 19$\pm2$ (119) & \nodata & M \\
V351 Pup & 6.5 (120) & 2448617.5 (120) & 16 (121) & \nodata & 0.72$\pm0.1$ (122) & 6.2e+21 & 0.1182 (123) & 2.7$\pm0.7$ (122) & N & \nodata \\
{\bf V382 Nor} & 8.9 (124) & 2453447.5 (124) & 12 (40) & 1850 (23) & \nodata & 1.7e+22 & \nodata & \nodata & \nodata & \nodata \\
V382 Vel & 2.85 (125) & 2451320.5 (125) & 4.5 (126) & 2400 (126) & 0.05: (126) & 3.4e+21  & 0.146126 (127) & 1.68$\pm0.3$ (126) & N & \nodata \\
{\bf V407 Cyg} & 6.8 (128) & 2455266.314 (128) & 5.9 (129) & 2760 (129) & 0.5$\pm0.05$ (130) & 8.8e+21 & 15595 (131) & 2.7 (131) & \nodata & Y \\
{\bf V458 Vul} & 8.24 (132) & 2454322.39 (132) & 7 (133) & 1750 (134) & 0.6 (135) & 3.6e+21 & 0.06812255 (136) & 8.5$\pm1.8$ (133) & N (135) & \nodata \\
{\bf V459 Vul} & 7.57 (137) & 2454461.5 (137) & 18 (138) & 910 (139) & 1.0 (140) & 5.5e+21  & \nodata & 3.65$\pm1.35$ (138) & Y (140) & \nodata \\
V4633 Sgr & 7.8 (141) & 2450895.5 (141) & 19$\pm3$ (142) & 1700 (143) & 0.21 (142) & 1.4e+21  & 0.125576 (144) & 8.9$\pm2.5$ (142) & N & \nodata \\
{\bf V4643 Sgr} & 8.07 (145) & 2451965.867 (145) & 4.8 (146) & 4700 (147) & 1.67 (148) & 1.4e+22 & \nodata & 3 (148) & N & \nodata \\
{\bf V4743 Sgr} & 5.0 (149) & 2452537.5 (149) & 9 (150) & 2400 (149) & 0.25 (151) & 1.2e+21 & 0.281 (152) & 3.9$\pm0.3$ (151) & N & \nodata \\
{\bf V4745 Sgr} & 7.41 (153) & 2452747.5 (153) & 8.6 (154) & 1600 (155) & 0.1 (154) & 9.0e+20  & 0.20782 (156) & 14$\pm5$ (154) & \nodata & \nodata \\
{\bf V476 Sct} & 10.3 (157) & 2453643.5 (157) & 15 (158) & \nodata & 1.9 (158) & 1.2e+22  & \nodata & 4$\pm1$ (158) & M (159) & \nodata \\
{\bf V477 Sct} & 9.8 (160) & 2453655.5 (160) & 3 (160) & 2900 (161) & 1.2: (162) & 4e+21  & \nodata & \nodata & M (163) & \nodata \\
{\bf V5114 Sgr} & 8.38 (164) & 2453081.5 (164) & 11 (165) & 2000 (23) & \nodata & 1.5e+21  & \nodata & 7.7$\pm0.7$ (165) & N (166) & \nodata \\
{\bf V5115 Sgr} & 7.7 (167) & 2453459.5 (167) & 7 (40) & 1300 (168) & 0.53 (169) & 2.3e+21  & \nodata & \nodata & N (169) & \nodata \\
{\bf V5116 Sgr} & 8.15 (170) & 2453556.91 (170) & 6.5 (171) & 970 (172) & 0.25 (173) & 1.5e+21 & 0.1238 (171) & 11$\pm3$ (173) & N (174) & \nodata \\
{\bf V5558 Sgr} & 6.53 (175) & 2454291.5 (175) & 125 (176) & 1000 (177) & 0.80 (178) & 1.6e+22  & \nodata & 1.3$\pm0.3$ (176) & N (179) & \nodata \\
{\bf V5579 Sgr} & 5.56 (180) & 2454579.62 (180) & 7: & 1500 (23) & 1.2 (181) & 3.3e+21 & \nodata & \nodata & Y (181) & \nodata \\
{\bf V5583 Sgr} & 7.43 (182) & 2455051.07 (182) & 5: & 2300 (182) & 0.39 (30) & 2.0e+21 & \nodata & 10.5 & \nodata & \nodata \\
{\bf V574 Pup} & 6.93 (183) & 2453332.22 (183) & 13 (184) & 2800 (184) & 0.5$\pm0.1$  & 6.2e+21 & \nodata & 6.5$\pm1$  & M (185) & \nodata \\
{\bf V597 Pup} & 7.0 (186) & 2454418.75 (186) & 3: & 1800 (187) & 0.3 (188) & 5.0e+21  & 0.11119 (189) & \nodata & N (188) & \nodata \\
{\bf V598 Pup} & 3.46 (14) & 2454257.79 (14) & 9$\pm1$ (190) & \nodata & 0.16 (190) & 1.4e+21 & \nodata & 2.95$\pm0.8$ (190) & \nodata & \nodata \\
{\bf V679 Car} & 7.55 (191) & 2454797.77 (191) & 20: & \nodata & \nodata & 1.3e+22  & \nodata & \nodata & \nodata & \nodata \\
{\bf V723 Cas} & 7.1 (192) & 2450069.0 (192) & 263 (2) & 600 (193) & 0.5 (194) & 2.35e+21  & 0.69 (195) & 3.86$\pm0.23$ (196) & N & \nodata \\
V838 Her & 5 (197) & 2448340.5 (197) & 2 (198) & \nodata & 0.5$\pm0.1$ (198) & 2.6e+21  & 0.2975 (199) & 3$\pm1$ (198) & Y (200) & \nodata \\
{\bf XMMSL1 J06} & 12 (201) & 2453643.5 (202) & 8$\pm2$ (202) & \nodata & 0.15 (203) & 8.7e+20 & \nodata & 50 & \nodata & \nodata \\
\enddata
\end{deluxetable*}
\end{longrotatetable}

A handy "cheat sheet" that provides the necessary LaTeX to produce 17 
different types of tables is available at \url{http://journals.aas.org/authors/aastex/aasguide.html#table_cheat_sheet}.

\section{IAU recommendations for nominal units \label{nominal}}

The IAU 2015 resolution B3 defines nominal solar and planetary values by
establishing conversions between solar and planetary values and SI units.
The rational and specifications are given in \citet{2016AJ....152...41P}.
The recommended nominal conversion constants for LaTeX have been
incorporate into v6.3 to help authors follow the IAU resolution.

The general commands take this form:

\vskip12pt
\begin{center}
\begin{tabular}{@{\vrule height 14pt depth 6pt width0pt}lll}
Command&Example&Results\\
\verb+\nom{}+&\verb+\nom{Q}+&\nom{Q}\\
\verb+\Eenom{}+&\verb+\Eenom{Q}+&\Eenom{Q}\\
\verb+\Epnom{}+&\verb+\Epnom{Q}+&\Epnom{Q}\\
\verb+\Jenom{}+&\verb+\Jenom{Q}+&\Jenom{Q}\\
\verb+\Jpnom{}+&\verb+\Jpnom{Q}+&\Jpnom{Q}\\
\end{tabular}
\end{center}
\vskip12pt

which can be used for any units the author requires. Examples of 
the most common uses would be:

\vskip12pt
\begin{tabular}{@{\vrule height 14pt depth 6pt width 0pt}llllp{3in}}
1.&\verb+\nom{(GM)}+& \nom{(GM)} &=& nominal solar mass parameter\\
2.&\verb+\nom{R}+&\nom{R} &=& nominal solar radius\\
3.&\verb+\nom{S}+& \nom{S}&=&  nominal total solar irradiance\\
4.&\verb+\nom{L}+& \nom{L}  &=&nominal solar luminosity\\
\end{tabular}
\vskip12pt

AASTeX v6.3 also contains specific commands for other commonly used 
units. These are:

\vskip24pt
\begin{tabular}{@{\vrule height 14pt depth 6pt width 0pt}llllp{3in}}
1.&\verb+\nomSolarEffTemp+& \nomSolarEffTemp&=& nominal solar effective temperature\\
2.&\verb+\nomTerrEqRadius+&\nomTerrEqRadius  &=& nominal terrestrial
equatorial radius\\
&\verb+\nomTerrPolarRadius+ &\nomTerrPolarRadius &=& nominal
terrestrial polar radius\\
&\verb+\nomTerrEqRadius+&\nomTerrEqRadius&& should be used if equatorial
vs.~polar radius is not explicitly specified.\\
3.&\verb+\nomJovianEqRadius+&\nomJovianEqRadius&=& nominal one-bar equatorial radii of
Jupiter\\
&\verb+\nomJovianPolarRadius+&\nomJovianPolarRadius &=& nominal polar radii of Jupiter\\
&\verb+\nomJovianEqRadius+&\nomJovianEqRadius&& should be used if Jovian equatorial
vs.~polar radius is not explicitly specified.\\
4.&\verb+\nomTerrMass+ &\nomTerrMass &=& nominal terrestrial mass
parameter\\
&\verb+\nomJovianMass+ &\nomJovianMass &=& nominal Jovian mass parameter\\
\end{tabular}
\vskip12pt

All of these commands work equally well in text and math mode.

%% For this sample we use BibTeX plus aasjournals.bst to generate the
%% the bibliography. The sample63.bib file was populated from ADS. To
%% get the citations to show in the compiled file do the following:
%%
%% pdflatex sample63.tex
%% bibtext sample63
%% pdflatex sample63.tex
%% pdflatex sample63.tex
